# Supplementary material for: Exact Hybrid Covariance Thresholding for Joint Graphical Lasso
Source: arXiv:1503.02128 source file (2015-06-18)
Supplement: Supplementary file 1 [file Supp_Figure_.pdf]

# Supplementary Material: Figures and Tables

## 1. Non-uniform partition example

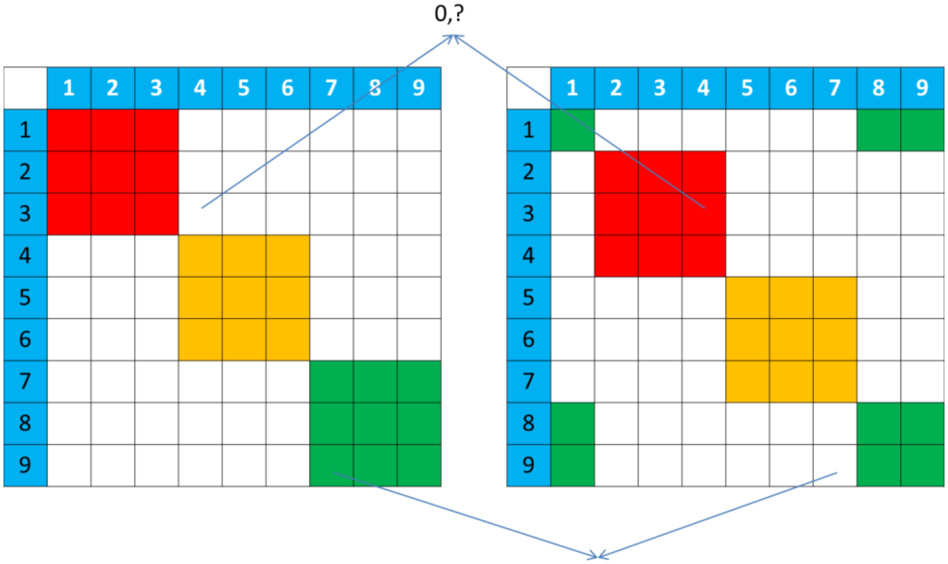


Figure S1: Illustration of a non-uniform partition. White color indicates zero entries detected by covariance thresholding. Entries with the same color other than white belong to the same group.

## 2. Comparison of hybrid, class-specific and global thresholding strategies

In Figure S2, both global and class-specific covariance thresholding fail to decompose the variable set into smaller subsets. The parameters used are $\lambda_1 = 0.04$ and $\lambda_2 = 0.02$. Global thresholding can set entries (1,2) and (2,1) to zero, but cannot split the variable set into disjoint subsets. Class-specific thresholding sets entries (1,3) and (3,1) to zero for the first class and entries (2,3) and (3,2) to zero for the second class, respectively, but cannot split the problem into subproblems either. Only the hybrid thresholding can split the matrices into submatrices.

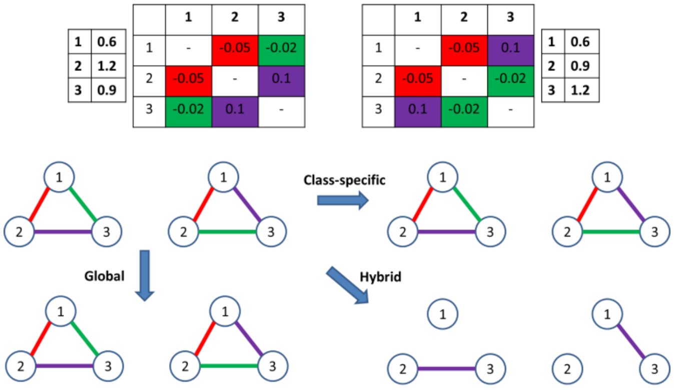


Figure S2: Comparison of three thresholding strategies. The dataset contains 2 slightly different classes and 3 variables. The two sample covariance matrices are shown on the top of the figure. The parameters used are $\lambda_1 = 0.04$ and $\lambda_2 = 0.02$.

## 3. Model Selection for Synthetic Data

We run the plain ADMM without screening using different values of the two hyper-parameters $\lambda_1$ and $\lambda_2$, and then compute the total absolute difference between the true precision matrices and the estimated values over all the classes. The difference on the three of data types is averaged and listed in the below table. We choose the values of the hyper-parameters to minimize the absolute error.

Table S1: Impact of hyper-parameters $\lambda_1$ and $\lambda_2$ on the three types of data ($p = 1000, K = 10$)

| $\lambda_2$ \ $\lambda_1$ | 0.0078 | 0.0082 | 0.0086 | 0.009 | 0.0094 |
|---|---|---|---|---|---|
| 0.0005 | 84.6 | 84.1 | 83.4 | 84.1 | 85.2 |
| 0.001 | 85.4 | 82.5 | 76.7 | 90.2 | 108.8 |
| 0.0015 | 92.4 | 81.3 | 80.6 | 99.4 | 117.9 |

According to the table, for $p = 1000$, we use ($\lambda_1 = 0.009, \lambda_2 = 0.0005$), ($\lambda_1 = 0.0086, \lambda_2 = 0.001$) and ($\lambda_1 = 0.0082, \lambda_2 = 0.0015$), respectively. Similarly, for $p = 10000$, we use ($\lambda_1 = 0.009, \lambda_2 = 0.0025$), ($\lambda_1 = 0.0094, \lambda_2 = 0.002$) and ($\lambda_1 = 0.0098, \lambda_2 = 0.0015$), respectively.

## 4. Convergence of our covariance thresholding algorithm on Synthetic Data

We compare the convergence property of our HADMM with the plain ADMM (i.e., no screening used). In terms of the objective function value, both HADMM and ADMM quickly yield similar values, as shown in Figures S3-S5. In terms of the gap between the primal and dual variables, our HADMM is much better than the other three methods.

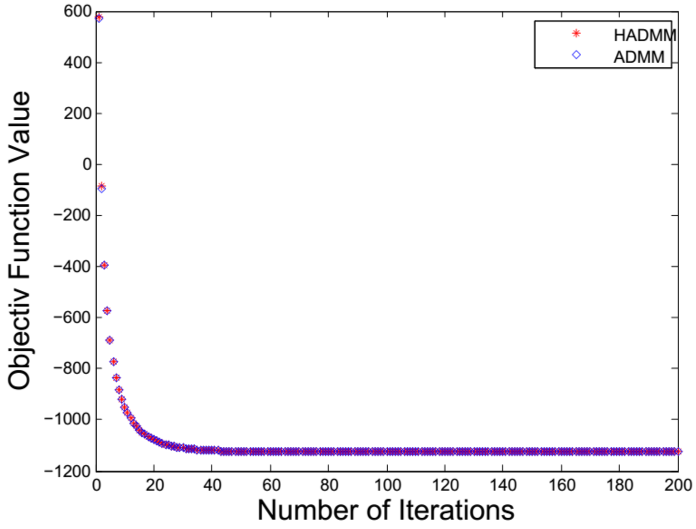


Figure S3. Objective function values of HADMM and ADMM vs. the number of iterations on a type A dataset (two classes, p=1000, $\lambda_1 = 0.009, \lambda_2 = 0.0005$ ).

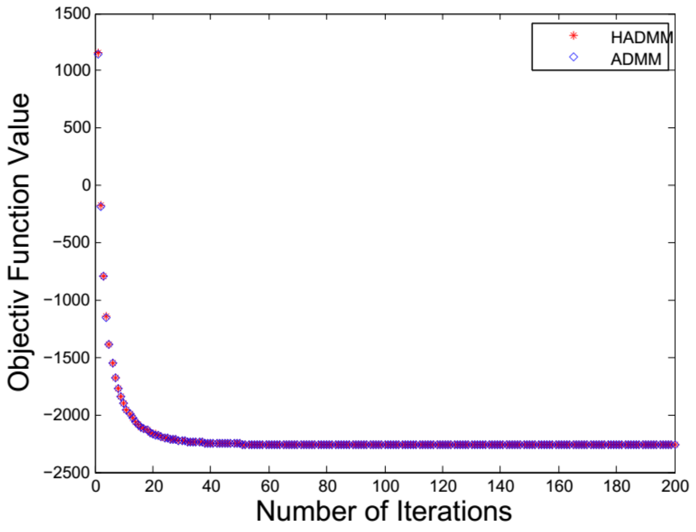


Figure S4. Objective function values of HADMM and ADMM vs. the number of iterations on a type B dataset (four classes, p=1000, $\lambda_1 = 0.0086, \lambda_2 = 0.001$ ).

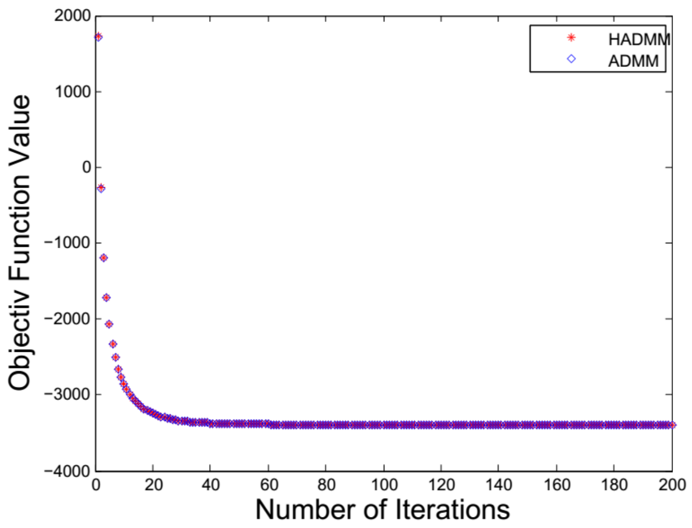


Figure S5. Objective function values of HADMM and ADMM vs. the number of iterations on a type C dataset (six classes, p=1000, $\lambda_1 = 0.0082, \lambda_2 = 0.0015$ ).

## 5. Estimated Computational Complexity of Eigen-decomposition

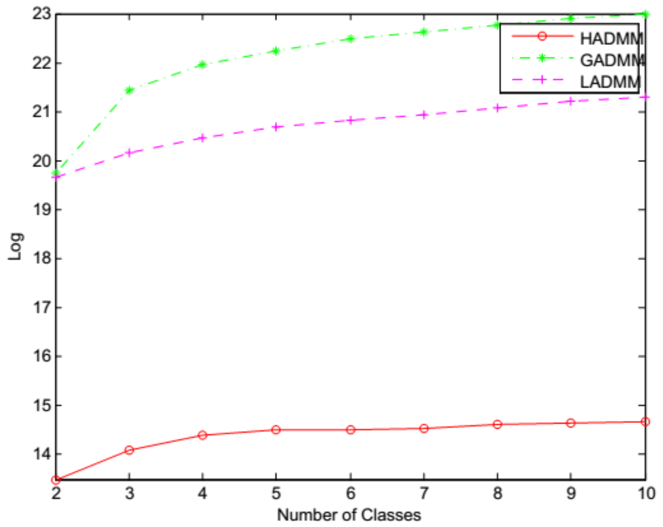


Figure S6: Estimated computational complexity of matrix eigen-decomposition in the HADMM, LADMM and GADMM algorithms (type A, $p = 1000$, $\lambda_1 = 0.009, \lambda_2 = 0.0005$)

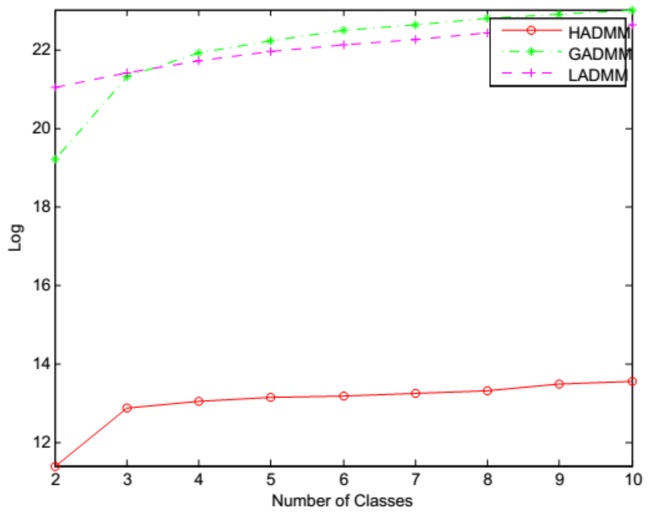


Figure S7: Estimated computational complexity of matrix eigen-decomposition in the HADMM, LADMM and GADMM algorithms (type A, $p = 1000$, $\lambda_1 = 0.0086, \lambda_2 = 0.001$)

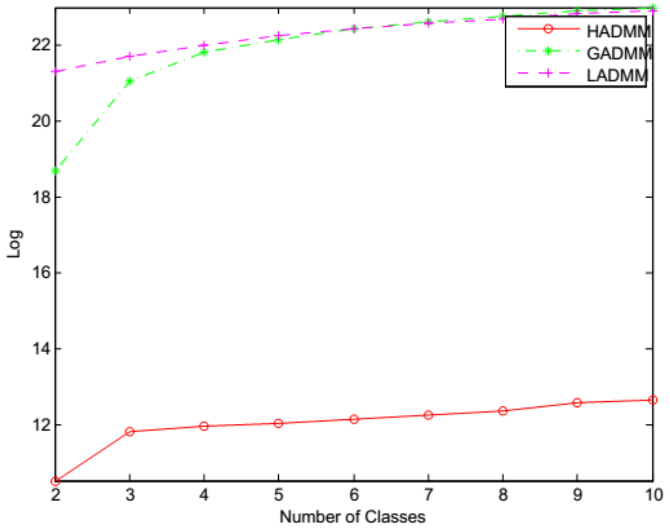


Figure S8: Estimated computational complexity of matrix eigen-decomposition in the HADMM, LADMM and GADMM algorithms (type A, $p = 1000$, $\lambda_1 = 0.0082, \lambda_2 = 0.0015$)

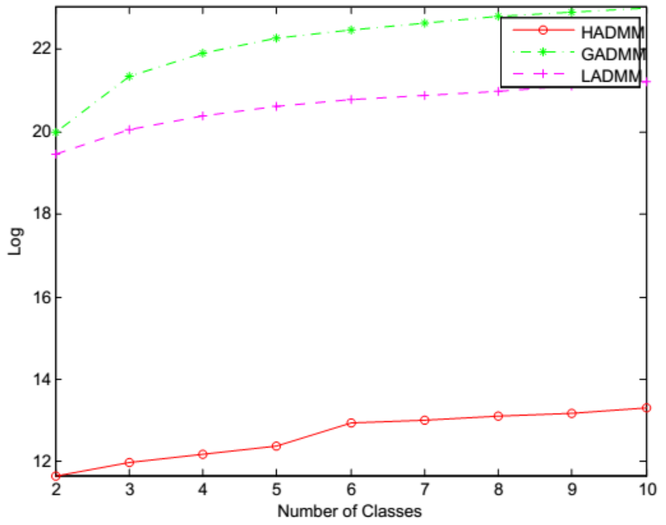


Figure S9: Estimated computational complexity of matrix eigen-decomposition in the HADMM, LADMM and GADMM algorithms (type B, $p = 1000$, $\lambda_1 = 0.009, \lambda_2 = 0.0005$)

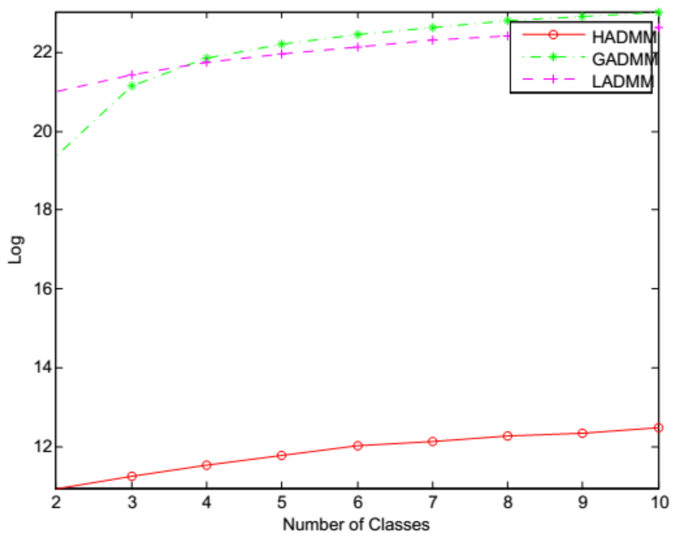


Figure S10: Estimated computational complexity of matrix eigen-decomposition in the HADMM, LADMM and GADMM algorithms (type B, $p = 1000$, $\lambda_1 = 0.0086, \lambda_2 = 0.001$)

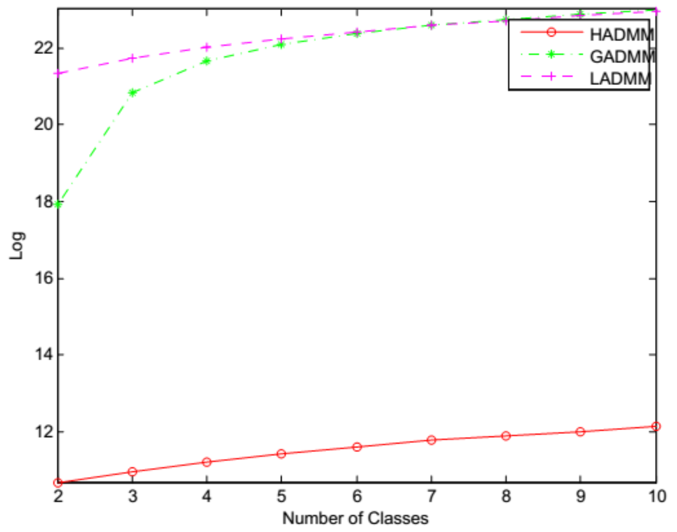


Figure S11: Estimated computational complexity of matrix eigen-decomposition in the HADMM, LADMM and GADMM algorithms (type B, $p = 1000$, $\lambda_1 = 0.0082, \lambda_2 = 0.0015$)

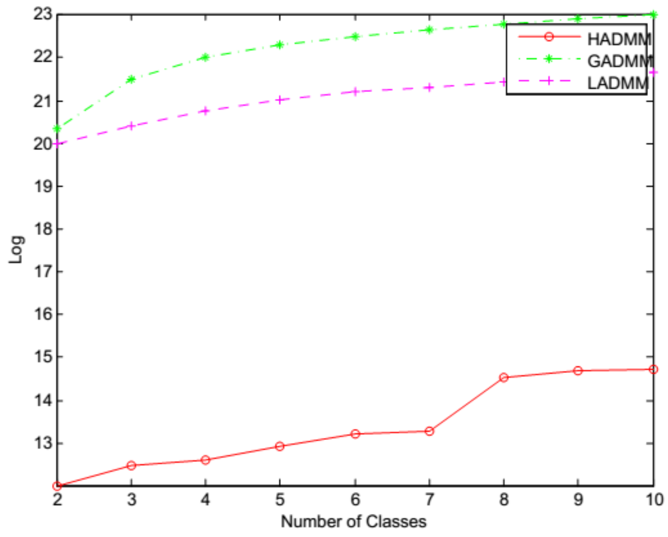


Figure S12: Estimated computational complexity of matrix eigen-decomposition in the HADMM, LADMM and GADMM algorithms (type C, $p = 1000$, $\lambda_1 = 0.009, \lambda_2 = 0.0005$)

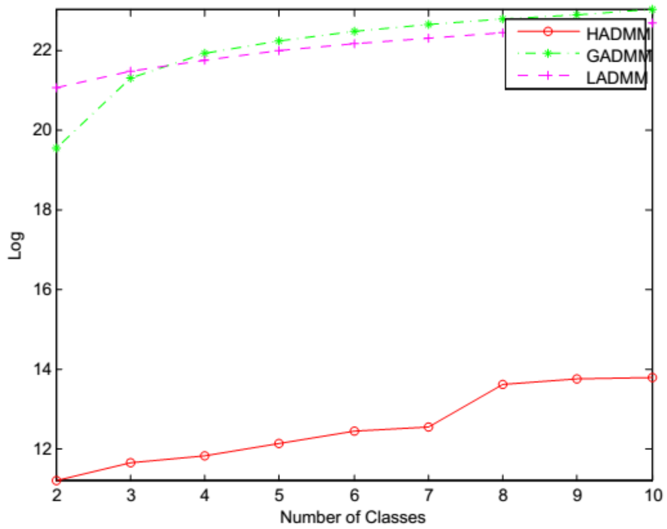


Figure S13: Estimated computational complexity of matrix eigen-decomposition in the HADMM, LADMM and GADMM algorithms (type C, $p = 1000$, $\lambda_1 = 0.0086, \lambda_2 = 0.001$)

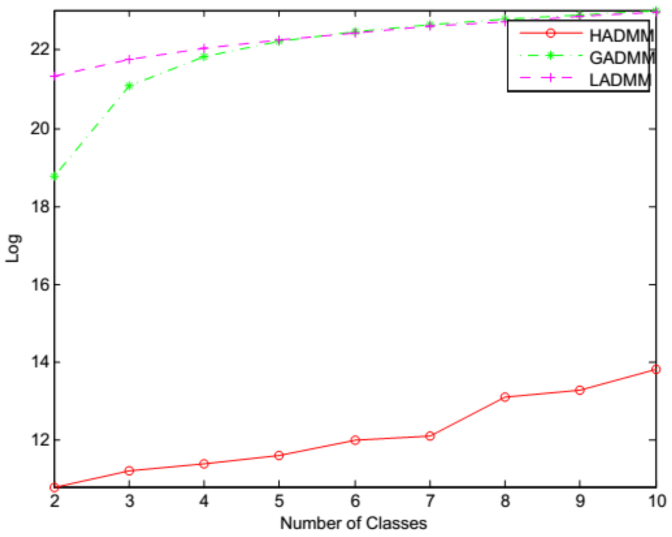


Figure S14: Estimated computational complexity of matrix eigen-decomposition in the HADMM, LADMM and GADMM algorithms (type C, $p = 1000$, $\lambda_1 = 0.0082, \lambda_2 = 0.0015$)

## 6. Experimental Results on Synthetic Data for $p = 10000$

This section includes all the figures summarizing the experiments on the synthetic dataset for $p = 10000$. We compare the running time and estimated computational complexity of the three screening-based ADMM methods HADMM, GADMM and LADMM and also the plain ADMM (i.e., no screening is used at all). We only test real data with 2 or 3 classes. The advantage of our non-uniform screening-based ADMM (i.e., HADMM) over ADMM, GADMM and LADMM is significant even when the number of classes is small. Below are our observations from the experiments:

1. As the number of classes increases to 6, HADMM is significantly faster than ADMM, LADMM and GADMM. In addition, HADMM is not very sensitive to the number of classes.
2. According to our estimation of the eigen-decomposition complexity, GADMM deteriorates very fast as the number of classes increase. This is not surprising since GADMM requires that all the classes use the same block structure, which leads to very large blocks when there are many classes.
3. Local screening strategy works poorly when p=10000. This implies that it is important to use the global information when p is large.

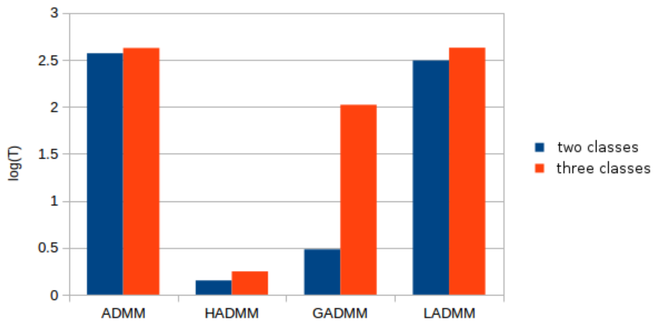


Figure S15: Running time of HADMM, ADMM, GADMM and LADMM on type A data ($p = 10000, \lambda_1 = 0.0098, \lambda_2 = 0.0015$). Y-axis is the logarithm of the number of minutes needed for one iteration.

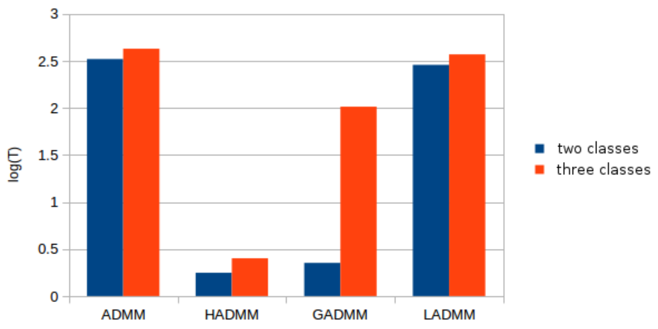


Figure S16: Running time of HADMM, ADMM, GADMM and LADMM on type A data ($p = 10000$, $\lambda_1 = 0.0094, \lambda_2 = 0.002$). Y-axis is the logarithm of the number of minutes needed for one iteration.

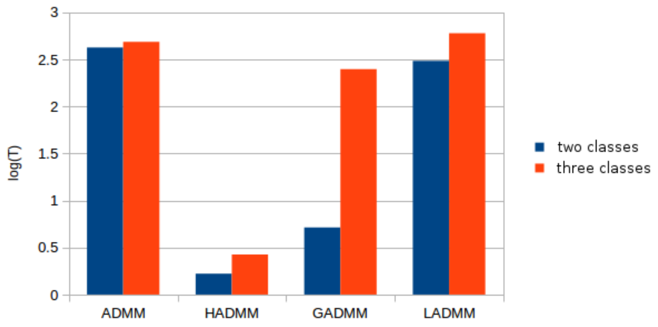


Figure S17: Running time of HADMM, ADMM, GADMM and LADMM on type A data ($p = 10000$, $\lambda_1 = 0.009, \lambda_2 = 0.0025$). Y-axis is the logarithm of the number of minutes needed for one iteration.

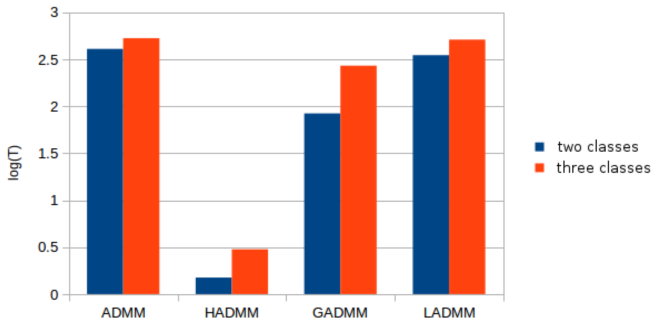


Figure S18: Running time of HADMM, ADMM, GADMM and LADMM on type B data ($p = 10000, \lambda_1 = 0.0098, \lambda_2 = 0.0015$). Y-axis indicates the logarithm of the number of minutes needed for one iteration.

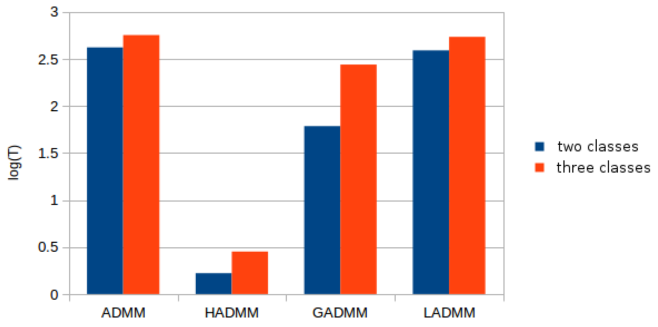


Figure S19: Running time of HADMM, ADMM, GADMM and LADMM on type B data ($p = 10000$, $\lambda_1 = 0.0094, \lambda_2 = 0.002$). Y-axis is the logarithm of the number of minutes needed for one iteration.

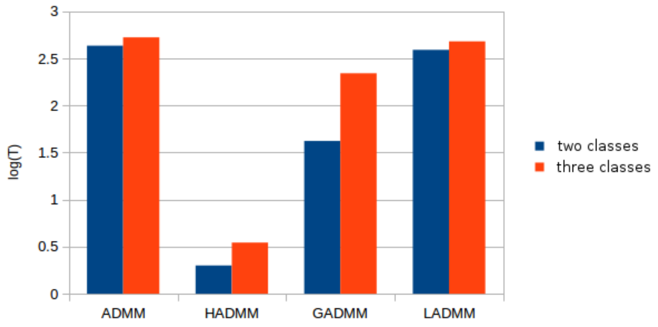


Figure S20: Running time of HADMM, ADMM, GADMM and LADMM on type B data ($p = 10000$, $\lambda_1 = 0.009, \lambda_2 = 0.0025$). Y-axis is the logarithm of the number of minutes needed for one iteration.

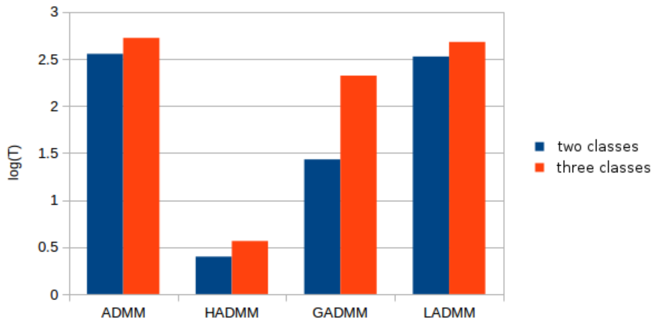


Figure S21: Running time of HADMM, ADMM, GADMM and LADMM on type C data ($p = 10000, \lambda_1 = 0.0098, \lambda_2 = 0.0015$). Y-axis is the logarithm of the number of minutes needed for one iteration.

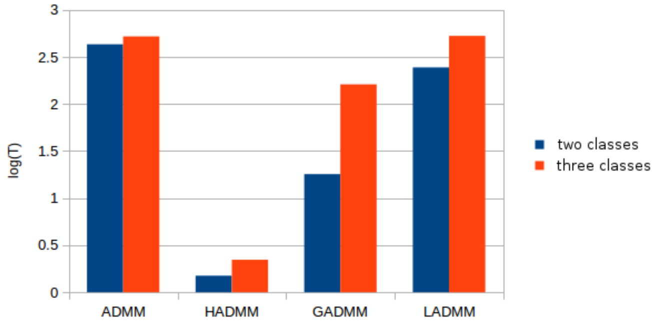


Figure S22: Running time of HADMM, ADMM, GADMM and LADMM on type C data ($p = 10000$, $\lambda_1 = 0.0094, \lambda_2 = 0.002$). Y-axis is the logarithm of the number of minutes needed for one iteration.

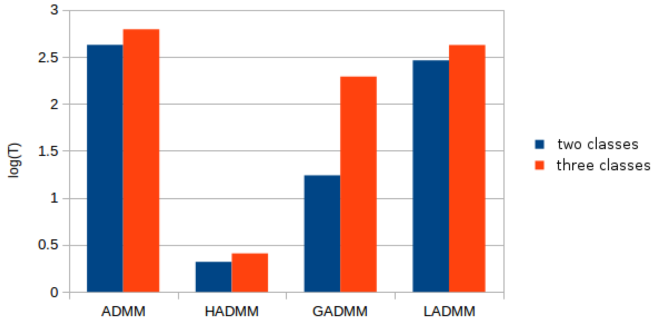


Figure S23: Running time of HADMM, ADMM, GADMM and LADMM on type C data ($p = 10000$, $\lambda_1 = 0.009, \lambda_2 = 0.0025$). Y-axis is the logarithm of the number of minutes needed for one iteration.

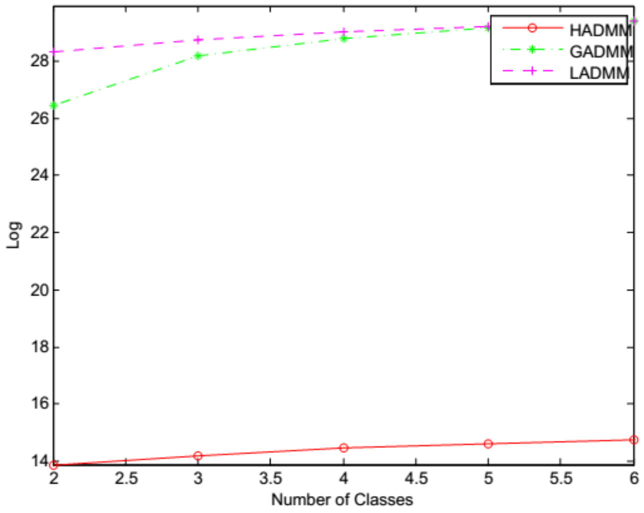


Figure S24: Estimated computational complexity of matrix eigen-decomposition in the HADMM, LADMM and GADMM algorithms (type A, $p = 10000, \lambda_1 = 0.0098, \lambda_2 = 0.0015$)

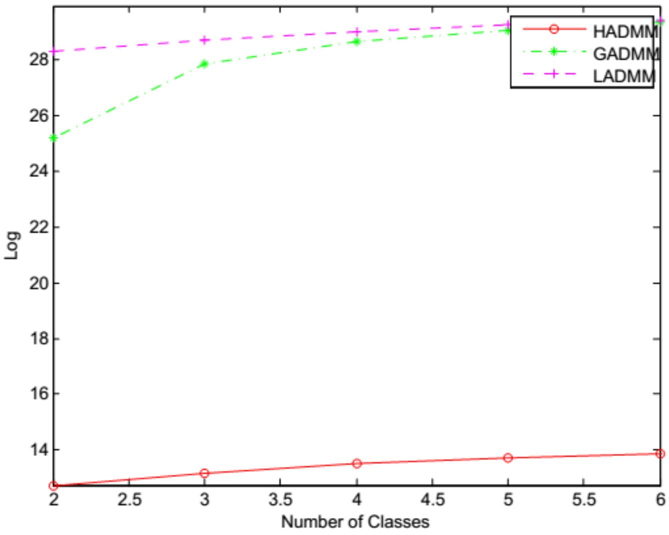

Figure S25: Estimated computational complexity of matrix eigen-decomposition in the HADMM, LADMM and GADMM algorithms (type A, $p = 10000$, $\lambda_1 = 0.0094, \lambda_2 = 0.002$)

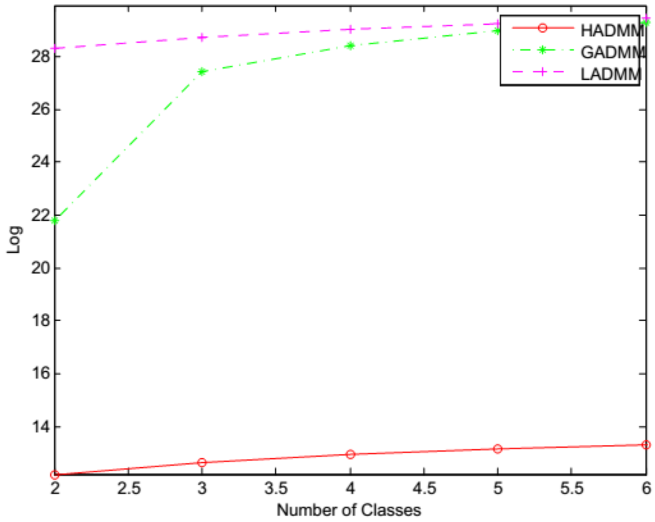

Figure S26: Estimated computational complexity of matrix eigen-decomposition in the HADMM, LADMM and GADMM algorithms (type A, $p = 10000$, $\lambda_1 = 0.009, \lambda_2 = 0.0025$)

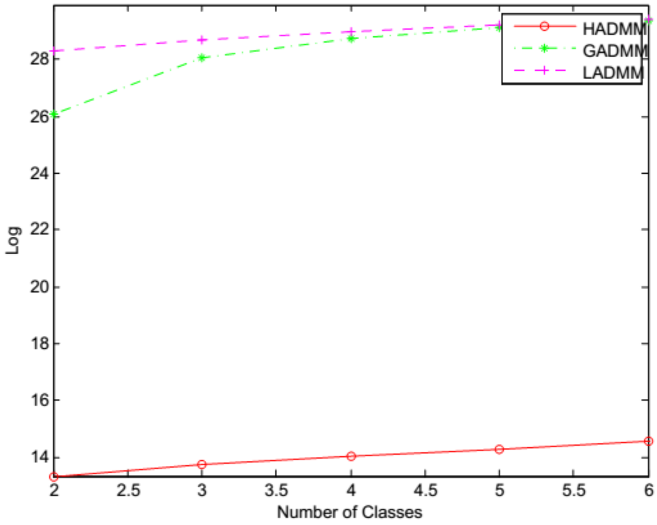


Figure S27: Estimated computational complexity of matrix eigen-decomposition in the HADMM, LADMM and GADMM algorithms (type B, $p = 10000, \lambda_1 = 0.0098, \lambda_2 = 0.0015$)

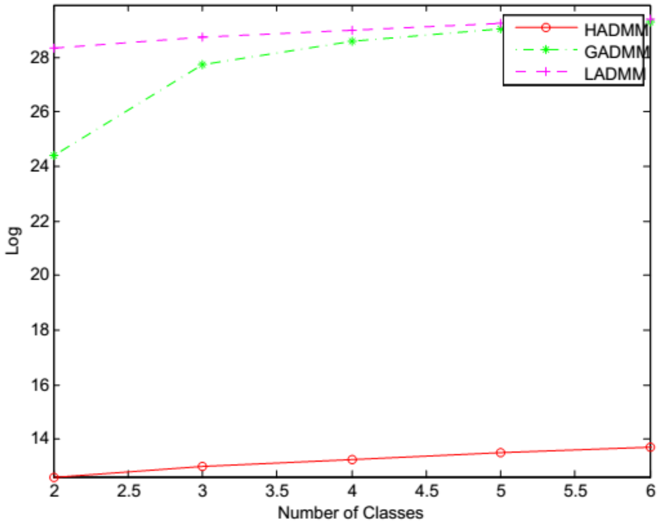


Figure S28: Estimated computational complexity of matrix eigen-decomposition in the HADMM, LADMM and GADMM algorithms (type B, $p = 10000$, $\lambda_1 = 0.0094, \lambda_2 = 0.002$)

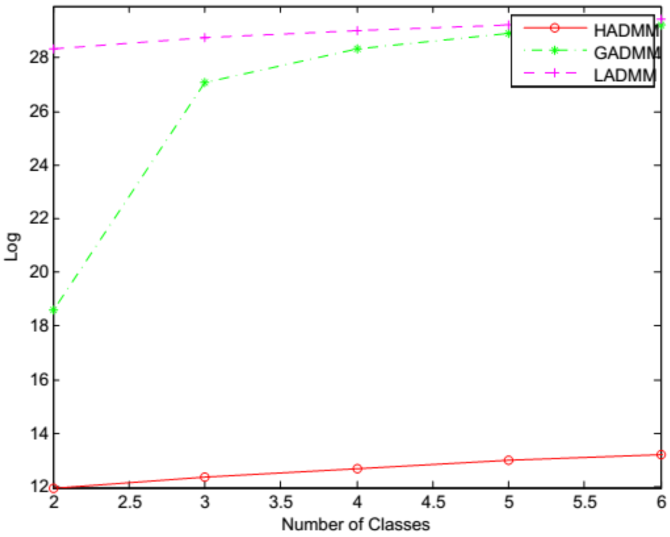


Figure S29: Estimated computational complexity of matrix eigen-decomposition in the HADMM, LADMM and GADMM algorithms (type B, $p = 10000$, $\lambda_1 = 0.009, \lambda_2 = 0.0025$)

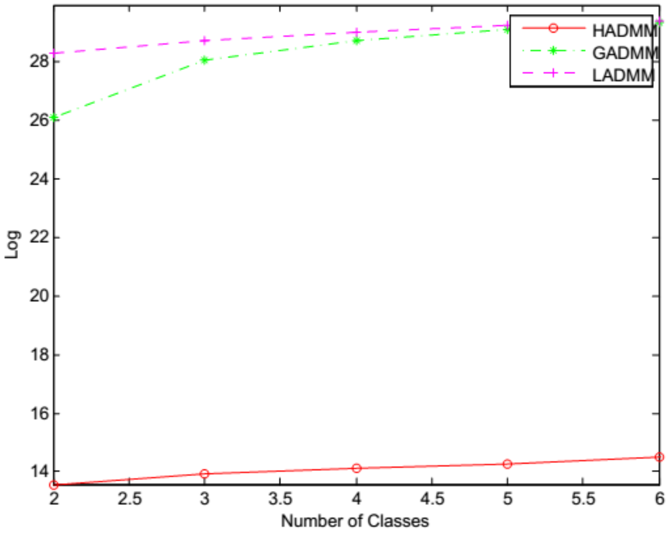


Figure S30: Estimated computational complexity of matrix eigen-decomposition in the HADMM, LADMM and GADMM algorithms (type C, $p = 10000, \lambda_1 = 0.0098, \lambda_2 = 0.0015$)

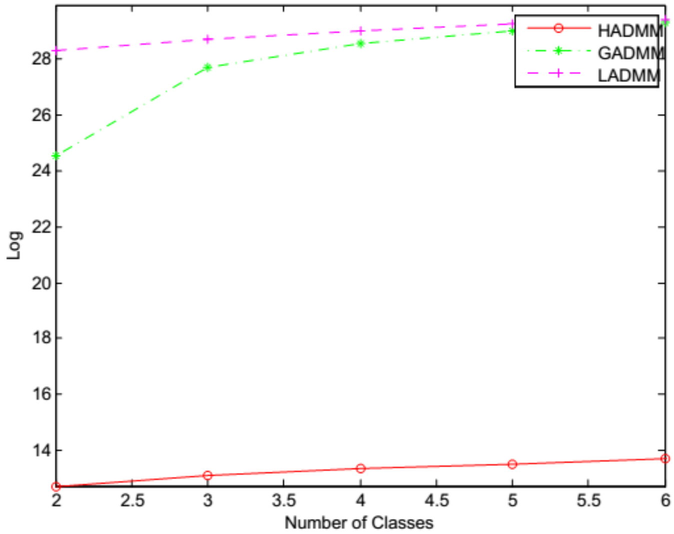


Figure S31: Estimated computational complexity of matrix eigen-decomposition in the HADMM, LADMM and GADMM algorithms (type C, $p = 10000$, $\lambda_1 = 0.0094, \lambda_2 = 0.002$)

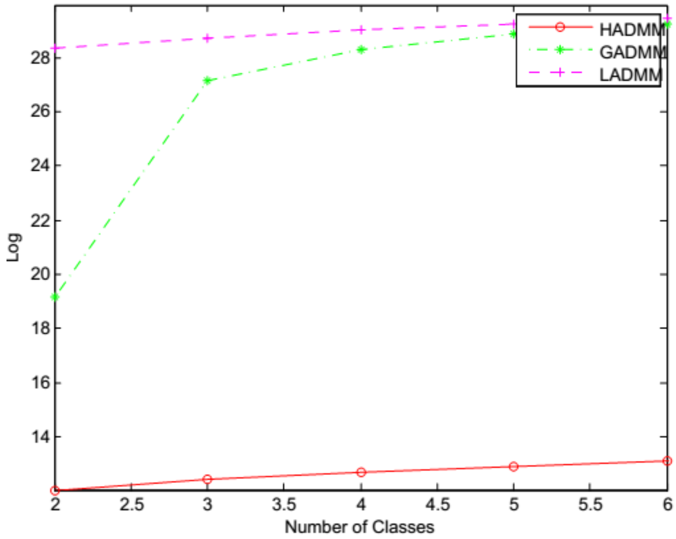


Figure S32: Estimated computational complexity of matrix eigen-decomposition in the HADMM, LADMM and GADMM algorithms (type C, $p = 10000$, $\lambda_1 = 0.009, \lambda_2 = 0.0025$)

## 7. Gene networks generated using different parameters

The following graphs are the networks generated by solving group graphical lasso using our hybrid covariance thresholding algorithm with parameters set to ($\lambda_1 = 0.1, \lambda_2 = 0.5$), ($\lambda_1 = 0.3, \lambda_2 = 0.1$) and ($\lambda_1 = 0.5, \lambda_2 = 0.01$), respectively. Due to space limit, we use Cytoscape (http://cytoscape.org/) to plot the network of the first 100 genes (ordered alphabetically). The full result is available upon request.

The following are the 100 genes used to plot the figures.

| A1CF | ABCA2 | ABCC9 | ABHD6 | ACADM |
|---|---|---|---|---|
| **A2M** | ABCA3 | ABCD1 | ABHD8 | ACADS |
| **A4GALT** | ABCA4 | ABCD2 | ABI1 | ACADSB |

| | | | | |
|---|---|---|---|---|
| **A4GNT** | ABCA5 | ABCD3 | ABI2 | ACADVL |
| **AAAS** | ABCA6 | ABCD4 | ABI3BP | ACAN |
| **AACS** | ABCA7 | ABCE1 | ABL1 | ACAP1 |
| **AADAC** | ABCB11 | ABCF1 | ABL2 | ACAP2 |
| **AAGAB** | ABCB4 | ABCF2 | ABLIM1 | ACAT1 |
| **AAK1** | ABCB6 | ABCF3 | ABLIM3 | ACAT2 |
| **AAMP** | ABCB7 | ABCG1 | ABO | ACBD3 |
| **AANAT** | ABCB8 | ABCG2 | ABP1 | ACBD4 |
| **AARS** | ABCB9 | ABCG4 | ABR | ACD |
| **AARSD1** | ABCC1 | ABCG5 | ABT1 | ACE |
| **AASDHPPT** | ABCC10 | ABHD10 | ABTB2 | ACE2 |
| **AASS** | ABCC2 | ABHD11 | ACAA2 | ACHE |
| **AATF** | ABCC3 | ABHD14A | ACACA | ACIN1 |
| **AATK** | ABCC4 | ABHD2 | ACACB | ACLY |
| **ABAT** | ABCC5 | ABHD3 | ACAD10 | ACN9 |
| **ABCA1** | ABCC6 | ABHD4 | ACAD8 | ACO1 |
| **ABCA12** | ABCC8 | ABHD5 | ACADL | ACO2 |

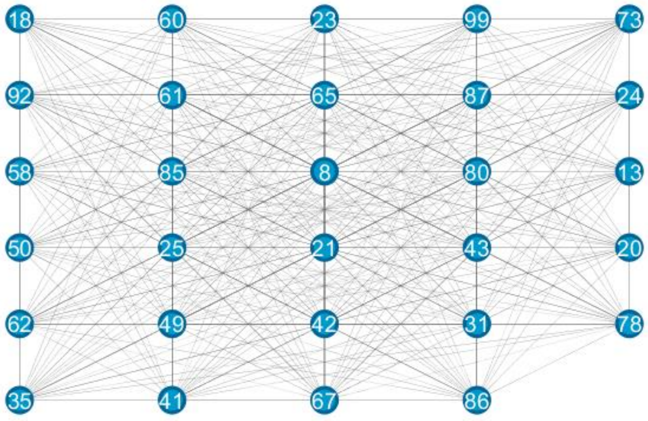


Figure S33: Network of the first 100 genes in the first class ($\lambda_1 = 0.1$, $\lambda_2 = 0.5$).

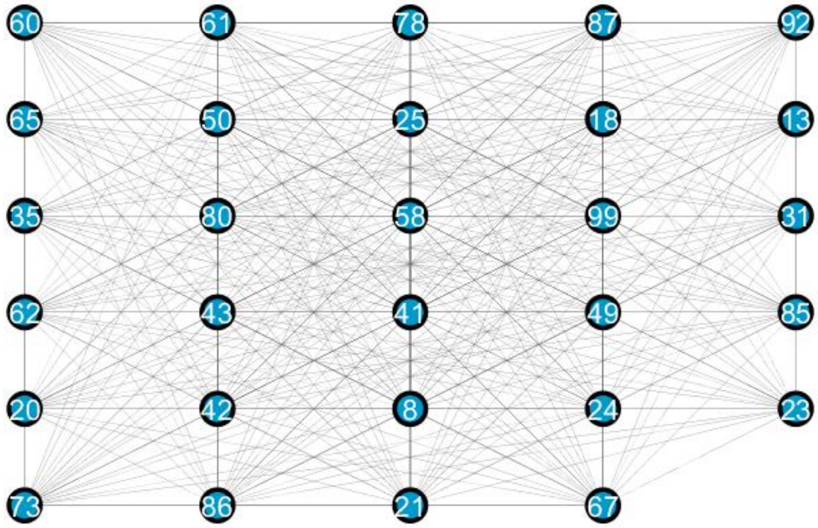


Figure S34: Network of the first 100 genes in the second class ($\lambda_1 = 0.1$, $\lambda_2 = 0.5$).

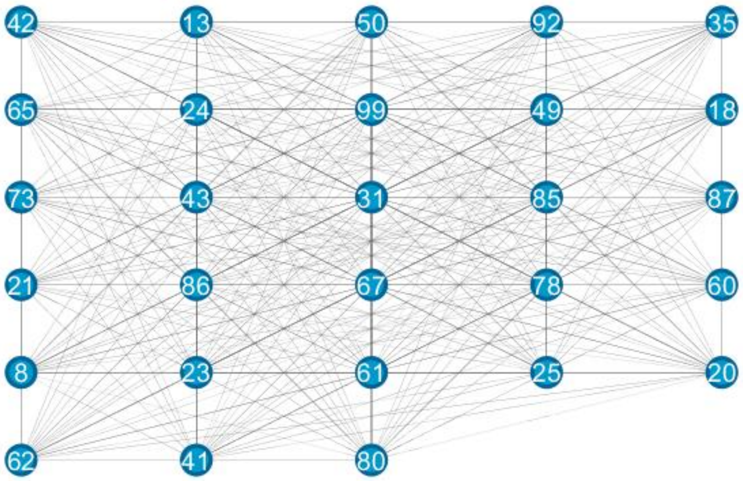


Figure S35: Network of the first 100 genes in the third class ($\lambda_1 = 0.1$, $\lambda_2 = 0.5$).

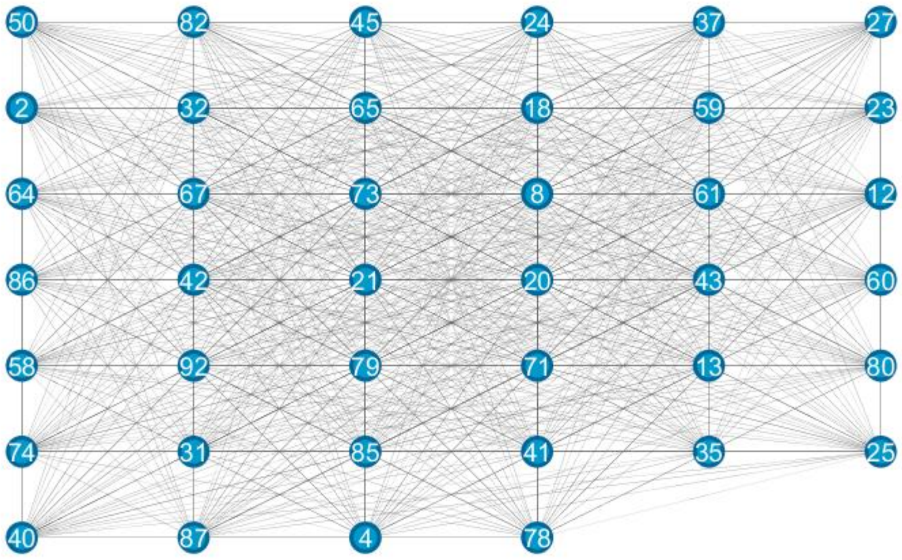


Figure S36: Network of the first 100 genes in the first class ($\lambda_1 = 0.3$, $\lambda_2 = 0.1$).

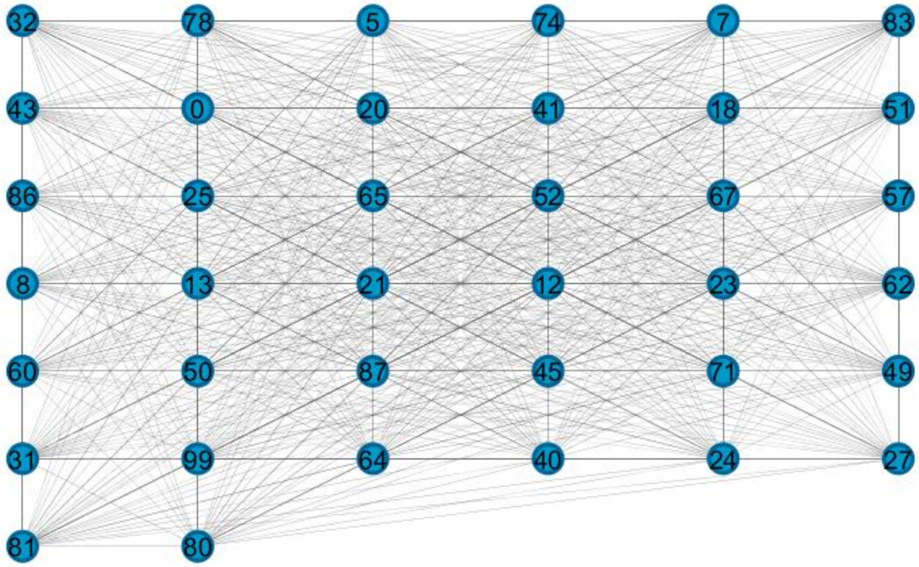


Figure S37: Network of the first 100 genes in the second class ($\lambda_1 = 0.3$, $\lambda_2 = 0.1$).

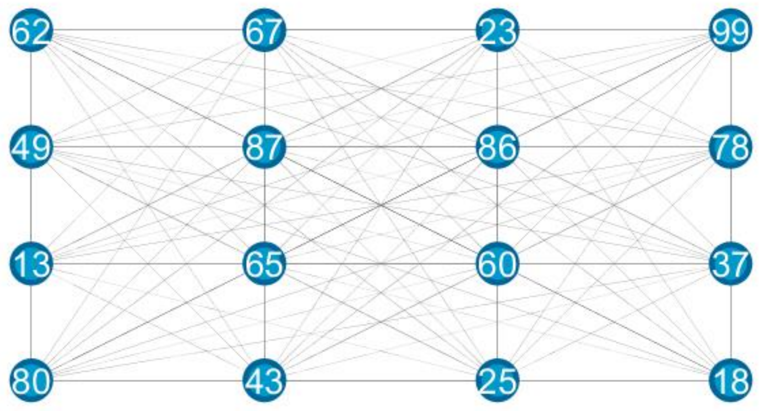


Figure S38: Network of the first 100 genes in the third class ($\lambda_1 = 0.3$, $\lambda_2 = 0.1$).

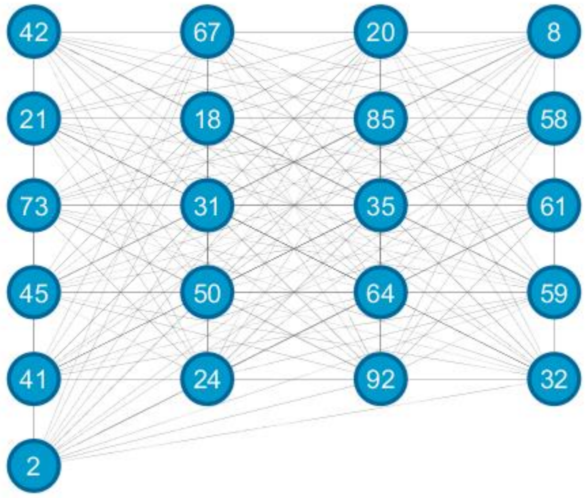


Figure S39: Network of the first 100 genes in the first class ($\lambda_1 = 0.5$, $\lambda_2 = 0.01$).

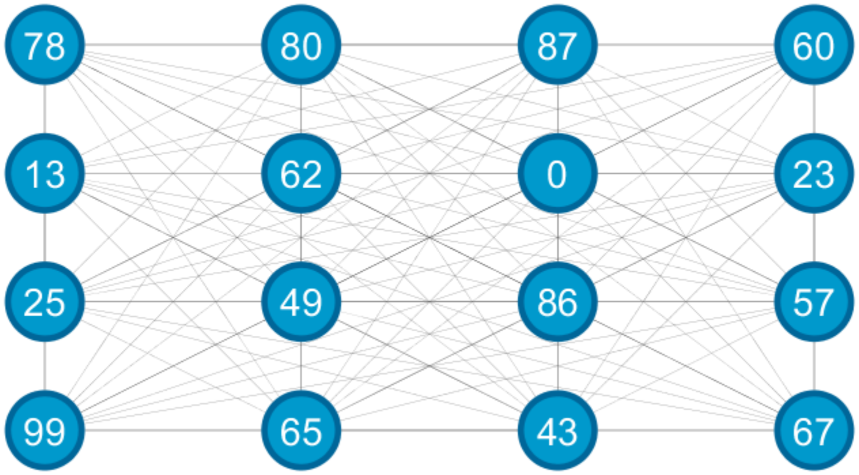


Figure S40: Network of the first 100 genes in the third class ($\lambda_1 = 0.5$, $\lambda_2 = 0.01$).

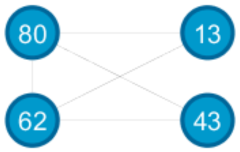


Figure S41: Network of the first 100 genes in the third class ($\lambda_1 = 0.5$, $\lambda_2 = 0.01$).
