# Supplementary material for: Exact Hybrid Covariance Thresholding for Joint Graphical Lasso
Source: arXiv:1503.02128 source file (2015-06-18)
Supplement: Supplementary file 2 [file Supp_Proof.pdf]

## SUPPLEMENTARY MATERIAL

The mathematical symbols used in the below proofs are defined in the main text.

### 1. Proof of Theorem 1

First, for any element  $\mathcal{H}_j$  in  $\mathcal{H}$ ,  $\mathbf{G}$  does not contain edges between  $\mathcal{H}_j$  and  $\mathcal{H} - \mathcal{H}_j$ . Otherwise, since  $\mathbf{G}$  is the mixing (or union) of all  $\mathbf{G}^{(k)}$ , there exists at least one graph  $\mathbf{G}^{(k)}$  such that it contains at least one edge between  $\mathcal{H}_j$  and  $\mathcal{H} - \mathcal{H}_j$ . Since  $\mathcal{H}_j$  is the union of some elements in  $\boxplus^{(k)}$ , this implies that there exist two different elements in  $\boxplus^{(k)}$  such that  $\mathbf{G}^{(k)}$  contains edges between them, which contradicts with the fact that  $\mathbf{G}^{(k)}$  does not contain edges between any two elements in  $\boxplus^{(k)}$ . That is,  $\mathcal{H}$  is feasible for graph  $\mathbf{G}$ .

Second, if  $\boxplus \preceq \mathcal{H}$  does not hold, then there is one element  $\boxplus_i$  in  $\boxplus$  and one element  $\mathcal{H}_j$  in  $\mathcal{H}$  such that  $\boxplus_i \cap \mathcal{H}_j \neq \emptyset$  and  $\boxplus_i - \mathcal{H}_j \neq \emptyset$ . Based on the above paragraph,  $\forall x \in \boxplus_i \cap \mathcal{H}_j$  and  $\forall y \in \boxplus_i - \mathcal{H}_j = \boxplus_i \cap (\mathcal{H} - \mathcal{H}_j)$ , we have  $\mathbf{E}_{x,y} = \mathbf{E}_{y,x} = 0$ . That is,  $\boxplus_i$  can be split into at least two disjoint subsets such that  $\mathbf{G}$  does not contain any edges between them. This contradicts with the fact that  $\boxplus_i$  corresponds to a connected component in graph  $\mathbf{G}$ .

### 2. Proof of Theorem 2

We now prove the following condition is **necessary** in order for a given non-uniform partition  $\{\mathcal{P}^{(1)}, \mathcal{P}^{(2)}, \dots, \mathcal{P}^{(K)}\}$  to be a feasible partition.

$$\begin{cases} \sum_{k=1}^K (|\mathcal{S}_{i,j}^{(k)}| - \lambda_1)_+^2 \leq \lambda_2^2, & \text{if } \forall k \in 1, \dots, K, \mathbf{I}_{i,j}^{(k)} = 0 \\ |\mathcal{S}_{i,j}^{(k)}| \leq \mathbf{Z}_{i,j}^{(k)}, & \text{if } \mathbf{I}_{i,j}^{(k)} = 0 \text{ and } \exists t \neq k, \mathbf{I}_{i,j}^{(t)} = 1 \end{cases} \quad (\text{A1})$$

Let  $\hat{\boldsymbol{\theta}}$  denote the optimal solution to the original group graphical lasso problem, then for any  $k$ , we have the following equation.

$$\hat{\boldsymbol{\theta}}^{(k)} = \min_{\boldsymbol{\theta}^{(k)} \geq 0} \{L(\boldsymbol{\theta}^{(k)}) + \lambda_1 \|\boldsymbol{\theta}^{(k)}\|_1 + 2\lambda_2 \sum_{1 \leq i < j \leq p} \sqrt{(\boldsymbol{\theta}_{i,j}^{(k)})^2 + \sum_{t \neq k} (\hat{\boldsymbol{\theta}}_{i,j}^{(t)})^2}\} \quad (\text{A2})$$

Let  $A^{(k)}(i, j) = \sum_{t \neq k} (\hat{\boldsymbol{\theta}}_{i,j}^{(t)})^2$ . The KKT condition of (A2) for any suitable pair  $(i, j)$  is:

$$\begin{cases} -(\boldsymbol{\theta}^{(k)})_{i,j}^{-1} + \mathbf{S}_{i,j}^{(k)} + \lambda_1 \Gamma(\boldsymbol{\theta}_{i,j}^{(k)}) + 2\lambda_2 \Gamma(\boldsymbol{\theta}_{i,j}^{(k)}) \\ -(\boldsymbol{\theta}^{(k)})_{j,i}^{-1} + \mathbf{S}_{j,i}^{(k)} + \lambda_1 \Gamma(\boldsymbol{\theta}_{j,i}^{(k)}) = 0, & \text{when } A^{(k)}(i, j) = 0 \\ -(\boldsymbol{\theta}^{(k)})_{i,j}^{-1} + \mathbf{S}_{i,j}^{(k)} + \lambda_1 \Gamma(\boldsymbol{\theta}_{i,j}^{(k)}) + 2\lambda_2 \frac{\boldsymbol{\theta}_{i,j}^{(k)}}{\sqrt{(\boldsymbol{\theta}_{i,j}^{(k)})^2 + A^{(k)}(i, j)}} \\ -(\boldsymbol{\theta}^{(k)})_{j,i}^{-1} + \mathbf{S}_{j,i}^{(k)} + \lambda_1 \Gamma(\boldsymbol{\theta}_{j,i}^{(k)}) = 0, & \text{when } A^{(k)}(i, j) \neq 0 \end{cases} \quad (\text{A3})$$

Since  $\boldsymbol{\theta}^{(k)}$  is symmetric, (A3) can be simplified as follows.

$$\begin{cases} -(\boldsymbol{\theta}^{(k)})_{i,j}^{-1} + \mathbf{S}_{i,j}^{(k)} + \lambda_1 \Gamma(\boldsymbol{\theta}_{i,j}^{(k)}) + \lambda_2 \Gamma(\boldsymbol{\theta}_{i,j}^{(k)}) = 0, & \text{when } A^{(k)}(i, j) = 0 \\ -(\boldsymbol{\theta}^{(k)})_{i,j}^{-1} + \mathbf{S}_{i,j}^{(k)} + \lambda_1 \Gamma(\boldsymbol{\theta}_{i,j}^{(k)}) + \lambda_2 \frac{\boldsymbol{\theta}_{i,j}^{(k)}}{\sqrt{(\boldsymbol{\theta}_{i,j}^{(k)})^2 + A^{(k)}(i, j)}} = 0, & \text{when } A^{(k)}(i, j) \neq 0 \end{cases} \quad (\text{A4})$$

Here  $\Gamma(\boldsymbol{\theta}_{i,j}^{(k)})$  denotes the sub-gradient of  $f(x) = |x|$  at point  $x = \boldsymbol{\theta}_{i,j}^{(k)}$ . Note that if  $\mathbf{I}_{i,j}^{(k)} = 0$ , then  $\boldsymbol{\theta}_{i,j}^{(k)} = 0$  and  $(\boldsymbol{\theta}^{(k)})_{i,j}^{-1} = 0$  since  $\boldsymbol{\theta}^{(k)}$  and  $(\boldsymbol{\theta}^{(k)})^{-1}$  share the same block structure.

Case 1: when  $\mathbf{I}_{i,j}^{(k)} = 0$ ,  $A^{(k)}(i, j) \neq 0$  and  $\exists t \neq k$ ,  $\mathbf{I}_{i,j}^{(t)} = 1$ , we have

$$-(\boldsymbol{\theta}^{(k)})_{i,j}^{-1} + \mathbf{s}_{i,j}^{(k)} + \lambda_1 \Gamma(\boldsymbol{\theta}_{i,j}^{(k)}) + \lambda_2 \frac{\boldsymbol{\theta}_{i,j}^{(k)}}{\sqrt{(\boldsymbol{\theta}_{i,j}^{(k)})^2 + A^{(k)}(i,j)}} = \mathbf{s}_{i,j}^{(k)} + \lambda_1 \Gamma(\boldsymbol{\theta}_{i,j}^{(k)}) = 0 \quad (\text{A5})$$

Since  $-1 \leq \Gamma(\boldsymbol{\theta}_{i,j}^{(k)}) \leq 1$ , we have

$$|\mathbf{s}_{i,j}^{(k)}| \leq \lambda_1. \quad (\text{A6})$$

Case 2: when  $\mathbf{I}_{i,j}^{(k)} = 0$ ,  $A^{(k)}(i,j) = 0$  and  $\exists t \neq k$ ,  $\mathbf{I}_{i,j}^{(t)} = 1$ , we have

$$-(\boldsymbol{\theta}^{(k)})_{i,j}^{-1} + \mathbf{s}_{i,j}^{(k)} + \lambda_1 \Gamma(\boldsymbol{\theta}_{i,j}^{(k)}) + \lambda_2 \Gamma(\boldsymbol{\theta}_{i,j}^{(k)}) = \mathbf{s}_{i,j}^{(k)} + (\lambda_1 + \lambda_2) \Gamma(\boldsymbol{\theta}_{i,j}^{(k)}) = 0 \quad (\text{A7})$$

Since  $-1 \leq \Gamma(\boldsymbol{\theta}_{i,j}^{(k)}) \leq 1$ , we have

$$|\mathbf{s}_{i,j}^{(k)}| \leq \lambda_1 + \lambda_2. \quad (\text{A8})$$

(A6) and (A8) can be merged as follows.

$$|\mathbf{s}_{i,j}^{(k)}| \leq \mathbf{z}_{i,j}^{(k)} = \lambda_1 + \lambda_2 \times \tau((\sum_{t \neq k} |\hat{\boldsymbol{\theta}}_{i,j}^{(t)}|) = 0) \quad (\text{A9})$$

Where  $\tau$  is the indicator function.

Case 3: when  $\mathbf{I}_{i,j}^{(k)} = 0$  for all  $k$ , we have the following  $K$  related equations:

$$\begin{cases} 0 + \mathbf{s}_{i,j}^{(1)} + \lambda_1 \Gamma(\boldsymbol{\theta}_{i,j}^{(1)}) + \lambda_2 \Psi_1(\boldsymbol{\theta}_{i,j}^{(1)}, \boldsymbol{\theta}_{i,j}^{(2)}, \dots, \boldsymbol{\theta}_{i,j}^{(K)}) = 0 \\ \dots \\ 0 + \mathbf{s}_{i,j}^{(K)} + \lambda_1 \Gamma(\boldsymbol{\theta}_{i,j}^{(K)}) + \lambda_2 \Psi_K(\boldsymbol{\theta}_{i,j}^{(1)}, \boldsymbol{\theta}_{i,j}^{(2)}, \dots, \boldsymbol{\theta}_{i,j}^{(K)}) = 0 \end{cases} \quad (\text{A10})$$

Here,  $\Psi_k(\boldsymbol{\theta}_{i,j}^{(1)}, \boldsymbol{\theta}_{i,j}^{(2)}, \dots, \boldsymbol{\theta}_{i,j}^{(K)})$  is the partial sub-gradient of  $\sqrt{\sum_{k=1}^K (\boldsymbol{\theta}_{i,j}^{(k)})^2}$  with respect to  $\boldsymbol{\theta}_{i,j}^{(k)}$ . Based upon (A10), we have

$$\begin{aligned} \sum_{k=1}^K \min |\mathbf{s}_{i,j}^{(k)} + \lambda_1 \Gamma(\boldsymbol{\theta}_{i,j}^{(k)})|_2^2 &\leq \sum_{k=1}^K |\mathbf{s}_{i,j}^{(k)} + \lambda_1 \Gamma(\boldsymbol{\theta}_{i,j}^{(k)})|_2^2 = \\ \sum_{k=1}^K \lambda_2^2 \Psi_k(\boldsymbol{\theta}_{i,j}^{(1)}, \boldsymbol{\theta}_{i,j}^{(2)}, \dots, \boldsymbol{\theta}_{i,j}^{(K)})^2 &\leq \lambda_2^2 \end{aligned} \quad (\text{A11})$$

Since  $\min |\mathbf{s}_{i,j}^{(k)} + \lambda_1 \Gamma(\boldsymbol{\theta}_{i,j}^{(k)})|_2^2 = (|\mathbf{s}_{i,j}^{(k)}| - \lambda_1)_+^2$ , we have

$$\sum_{k=1}^K (|\mathbf{s}_{i,j}^{(k)}| - \lambda_1)_+^2 \leq \lambda_2^2 \quad (\text{A12})$$

Combining (A9) and (A12), we have proved that (A1) is the necessary condition.

### 3. Proof of Theorem 3

Similar to the proof of Theorem 2, let  $\Gamma(x)$  denote the sub-gradient of  $f(x) = |x|$  and  $\Psi_k(\boldsymbol{\theta}_{i,j}^{(1)}, \boldsymbol{\theta}_{i,j}^{(2)}, \dots, \boldsymbol{\theta}_{i,j}^{(K)})$  the partial sub-gradient of  $\sqrt{\sum_{k=1}^K (\boldsymbol{\theta}_{i,j}^{(k)})^2}$  with respect to  $\boldsymbol{\theta}_{i,j}^{(k)}$  ( $1 \leq k \leq K$ ).

Given a non-uniform partition  $\mathcal{P} = \{\mathcal{P}^{(1)}, \mathcal{P}^{(2)}, \dots, \mathcal{P}^{(K)}\}$  and accordingly  $F^{(k)}(i)$ , we define a set of  $K$  positive definite matrices of size  $p \times p$  as follows.

$$\mathcal{C} = \{\boldsymbol{\theta} = \{\boldsymbol{\theta}^{(1)}, \boldsymbol{\theta}^{(2)}, \dots, \boldsymbol{\theta}^{(K)}\} \mid \boldsymbol{\theta}_{i,j}^{(k)} = 0 \text{ if } F^{(k)}(i) \neq F^{(k)}(j), 1 \leq k \leq K\} \quad (\text{A13})$$

Consider the following optimization problem:

$$\min_{\boldsymbol{\theta} \in \mathcal{C}} \sum_{k=1}^K L(\boldsymbol{\theta}^{(k)}) + \lambda_1 \sum_{k=1}^K \|\boldsymbol{\theta}^{(k)}\|_1 + 2\lambda_2 \sum_{1 \leq i < j \leq p} \sqrt{\sum_{k=1}^K (\boldsymbol{\theta}_{i,j}^{(k)})^2} \quad (\text{A14})$$

Since (A14) is convex, it has a unique optimal solution, denoted as  $\tilde{\boldsymbol{\theta}}$ . To prove this lemma, we just need to show that under condition (8),  $\tilde{\boldsymbol{\theta}}$  is the solution of the original group graphical lasso. This is equivalent to

showing that for any suitable pair  $(i, j)$ , by setting  $\Gamma(\tilde{\theta}_{i,j}^{(k)})$  and  $\Psi_k(\tilde{\theta}_{i,j}^{(1)}, \tilde{\theta}_{i,j}^{(2)}, \dots, \tilde{\theta}_{i,j}^{(K)})$  ( $1 \leq k \leq K$ ) appropriately, we can realize the following equations.

$$\begin{cases} -(\tilde{\theta}_{i,j}^{(1)})^{-1} + \mathbf{s}_{i,j}^{(1)} + \lambda_1 \Gamma(\tilde{\theta}_{i,j}^{(1)}) + \lambda_2 \Psi_1(\tilde{\theta}_{i,j}^{(1)}, \tilde{\theta}_{i,j}^{(2)}, \dots, \tilde{\theta}_{i,j}^{(K)}) = 0 \\ \dots \\ -(\tilde{\theta}_{i,j}^{(K)})^{-1} + \mathbf{s}_{i,j}^{(K)} + \lambda_1 \Gamma(\tilde{\theta}_{i,j}^{(K)}) + \lambda_2 \Psi_K(\tilde{\theta}_{i,j}^{(1)}, \tilde{\theta}_{i,j}^{(2)}, \dots, \tilde{\theta}_{i,j}^{(K)}) = 0 \end{cases} \quad (\text{A15})$$

$$\begin{cases} \sum_{k=1}^K \Psi_k^2(\tilde{\theta}_{i,j}^{(1)}, \tilde{\theta}_{i,j}^{(2)}, \dots, \tilde{\theta}_{i,j}^{(K)}) = 1 & \text{if } \sum_{k=1}^K |\tilde{\theta}_{i,j}^{(k)}| \neq 0 \\ \sum_{k=1}^K \Psi_k^2(\tilde{\theta}_{i,j}^{(1)}, \tilde{\theta}_{i,j}^{(2)}, \dots, \tilde{\theta}_{i,j}^{(K)}) \leq 1 & \text{if } \sum_{k=1}^K |\tilde{\theta}_{i,j}^{(k)}| = 0 \end{cases} \quad (\text{A16})$$

Case 1: when  $I_{i,j}^{(k)} \neq 0$  for all  $k$ , we already have the KKT conditions with form shown as (A15). As such, Eq. (A15) holds while (A16) is satisfied.

Case 2: when  $I_{i,j}^{(k)} = 0$  for all  $k$ , (A15) is equivalent to the following equations.

$$\begin{cases} 0 + \mathbf{s}_{i,j}^{(1)} + \lambda_1 \Gamma(\tilde{\theta}_{i,j}^{(1)}) + \lambda_2 \Psi_1(\tilde{\theta}_{i,j}^{(1)}, \tilde{\theta}_{i,j}^{(2)}, \dots, \tilde{\theta}_{i,j}^{(K)}) = 0 \\ \dots \\ 0 + \mathbf{s}_{i,j}^{(K)} + \lambda_1 \Gamma(\tilde{\theta}_{i,j}^{(K)}) + \lambda_2 \Psi_K(\tilde{\theta}_{i,j}^{(1)}, \tilde{\theta}_{i,j}^{(2)}, \dots, \tilde{\theta}_{i,j}^{(K)}) = 0 \end{cases} \quad (\text{A17})$$

By setting  $\mathbf{s}_{i,j}^{(k)} + \lambda_1 \Gamma(\tilde{\theta}_{i,j}^{(k)}) = \text{sgn}(\mathbf{s}_{i,j}^{(k)}) \times (|\mathbf{s}_{i,j}^{(k)}| - \lambda_1)_+$  and  $\Psi_k(\tilde{\theta}_{i,j}^{(1)}, \tilde{\theta}_{i,j}^{(2)}, \dots, \tilde{\theta}_{i,j}^{(K)}) = -\text{sgn}(\mathbf{s}_{i,j}^{(k)}) \times \frac{(|\mathbf{s}_{i,j}^{(k)}| - \lambda_1)_+}{\lambda_2}$  for  $1 \leq k \leq K$ , we can satisfy Eqs.(A16) and (A17). Eq.(A16) holds because of the following equation.

$$\sum_{k=1}^K \lambda_2^2 \Psi_k^2(\tilde{\theta}_{i,j}^{(1)}, \tilde{\theta}_{i,j}^{(2)}, \dots, \tilde{\theta}_{i,j}^{(K)}) = \sum_{k=1}^K (|\mathbf{s}_{i,j}^{(k)}| - \lambda_1)_+^2 \leq \lambda_2^2 \quad (\text{A18})$$

Thus, we can satisfy Eqs.(A15) and (A16) by setting  $\Gamma(\tilde{\theta}_{i,j}^{(k)})$  and  $\Psi_k(\tilde{\theta}_{i,j}^{(1)}, \tilde{\theta}_{i,j}^{(2)}, \dots, \tilde{\theta}_{i,j}^{(K)})$  appropriately.

Case 3: when there are two indices  $s$  and  $t$  ( $1 \leq s \neq t \leq K$ ), such that  $I_{i,j}^{(s)} = 0$  and  $I_{i,j}^{(t)} = 1$ . Without loss of generality, we assume that  $I_{i,j}^{(k)} = 0$  for  $k \leq a$  and  $I_{i,j}^{(k)} = 1$  for  $k > a$ .

Set  $\Gamma(\tilde{\theta}_{i,j}^{(k)}) = \frac{\mathbf{s}_{i,j}^{(k)}}{\lambda_1}$  and  $\Psi_k(\tilde{\theta}_{i,j}^{(1)}, \tilde{\theta}_{i,j}^{(2)}, \dots, \tilde{\theta}_{i,j}^{(K)}) = 0$  for  $k \leq a$  and we can satisfy Eqs. (A15) and (A16).

In summary, (A15) holds for all the three cases, so  $\tilde{\theta}$  is the solution of the original group graphical lasso.

#### 4. Proof of Theorem 4

We prove this theorem in two parts. In **Part I**, we prove that after executing the part before the **Repeat Loop** of our hybrid algorithm, the resultant partition is finer than any partition satisfying condition (8). In **Part II**, we prove that when the algorithm terminates, the resultant partition is still finer than any partition satisfying condition (8), and thus the resultant partition is the finest feasible partition satisfying condition (8) according to **Theorem 3**.

##### Part I.

Let  $\{\mathcal{O}^{(1)}, \mathcal{O}^{(2)}, \dots, \mathcal{O}^{(K)}\}$  denote any partition satisfying condition (8) stated in the main text. Let  $\{\mathcal{U}^{(1)}, \mathcal{U}^{(2)}, \dots, \mathcal{U}^{(K)}\}$  denote the non-uniform partition defined by the resultant  $\{\mathbf{I}^{(1)}, \mathbf{I}^{(2)}, \dots, \mathbf{I}^{(K)}\}$  before executing the **Repeat Loop** of our hybrid algorithm. We prove that  $\mathcal{U}^{(k)} \preceq \mathcal{O}^{(k)}$  holds for all  $k$  by contradiction as follows. If there exists one  $k$  such that  $\mathcal{U}^{(k)} \not\preceq \mathcal{O}^{(k)}$  does not hold, then there is one element  $\mathcal{U}_i^{(k)}$  in  $\mathcal{U}^{(k)}$  overlapping with at least two elements in  $\mathcal{O}^{(k)}$ . Suppose that  $\mathcal{U}_i^{(k)}$  overlaps with only two elements  $\mathcal{O}_j^{(k)}$  and  $\mathcal{O}_s^{(k)}$  in  $\mathcal{O}^{(k)}$  ( $s < j$ ), i.e.,

$$\mathcal{U}_i^{(k)} \cap \mathcal{O}_j^{(k)} \neq \emptyset \text{ and } \mathcal{U}_i^{(k)} \cap \mathcal{O}_s^{(k)} \neq \emptyset \quad (\text{A19})$$

Since  $\{\mathcal{O}^{(1)}, \mathcal{O}^{(2)}, \dots, \mathcal{O}^{(K)}\}$  satisfies condition (8), we have

$$\forall x \in \mathcal{O}_j^{(k)} \text{ and } \forall y \in \mathcal{O}_s^{(k)}, \sum_{k=1}^K (|\mathbf{S}_{x,y}^{(k)}| - \lambda_1)_+^2 \leq \lambda_2^2 \text{ or } |\mathbf{S}_{x,y}^{(k)}| \leq \lambda_1 \quad (\text{A20})$$

Combining (A19) and (A20), we have

$$\forall x \in \mathcal{U}_i^{(k)} \cap \mathcal{O}_j^{(k)} \text{ and } \forall y \in \mathcal{U}_i^{(k)} \cap \mathcal{O}_s^{(k)}, \sum_{k=1}^K (|\mathbf{S}_{x,y}^{(k)}| - \lambda_1)_+^2 \leq \lambda_2^2 \text{ or } |\mathbf{S}_{x,y}^{(k)}| \leq \lambda_1 \quad (\text{A21})$$

Under this scenario, all the edges between  $\mathcal{U}_i^{(k)} \cap \mathcal{O}_j^{(k)}$  and  $\mathcal{U}_i^{(k)} \cap \mathcal{O}_s^{(k)}$  would be removed by steps 2 and 3 of the **First For Loop** in our hybrid algorithm. This implies that  $\mathcal{U}_i^{(k)}$  can be further split into smaller subsets, which contradicts with the definition of  $\{\mathcal{U}^{(1)}, \mathcal{U}^{(2)}, \dots, \mathcal{U}^{(K)}\}$ .

Similarly, we can prove that  $\mathcal{U}_i^{(k)}$  cannot overlap with more than two elements of  $\mathcal{O}^{(k)}$ . As such,  $\mathcal{U}^{(k)} \preceq \mathcal{O}^{(k)}$  holds for all  $k$ .

## Part II.

Let  $\{\mathbf{I}^{(1)}, \mathbf{I}^{(2)}, \dots, \mathbf{I}^{(K)}\}_i$  denote the resultant  $\{\mathbf{I}^{(1)}, \mathbf{I}^{(2)}, \dots, \mathbf{I}^{(K)}\}$  after **Repeat Loop** has been executed  $i$  times and  $\{\mathcal{U}^{(1)}, \mathcal{U}^{(2)}, \dots, \mathcal{U}^{(K)}\}_i$  the non-uniform partition defined by  $\{\mathbf{I}^{(1)}, \mathbf{I}^{(2)}, \dots, \mathbf{I}^{(K)}\}_i$ . In **Part I**, we have proved that before executing **Repeat Loop**, the initial  $\{\mathcal{U}^{(1)}, \mathcal{U}^{(2)}, \dots, \mathcal{U}^{(K)}\}_0$  satisfies the following condition.

$$\mathcal{U}^{(k)} \preceq \mathcal{O}^{(k)} \text{ for } k = 1, \dots, K \quad (\text{A22})$$

Assuming  $\{\mathcal{U}^{(1)}, \mathcal{U}^{(2)}, \dots, \mathcal{U}^{(K)}\}_i$  satisfies (A22), we want to prove  $\{\mathcal{U}^{(1)}, \mathcal{U}^{(2)}, \dots, \mathcal{U}^{(K)}\}_{i+1}$  also satisfies (A22).

Our hybrid algorithm merges two groups (components) when executing the **Repeat Loop**. Let  $\mathcal{U}_a^{(k)}$  and  $\mathcal{U}_b^{(k)}$  be the two groups (components) to be merged. According to hybrid screening algorithm, there exist  $x' \in \mathcal{U}_a^{(k)}$  and  $y' \in \mathcal{U}_b^{(k)}$  such that condition (8) does not hold. We can prove that there exists one element  $\mathcal{O}_c^{(k)}$  in  $\mathcal{O}^{(k)}$  such that  $\mathcal{U}_a^{(k)} \subseteq \mathcal{O}_c^{(k)}$  and  $\mathcal{U}_b^{(k)} \subseteq \mathcal{O}_c^{(k)}$ . If this is not true, assume that there are two different elements  $\mathcal{O}_c^{(k)}$  and  $\mathcal{O}_d^{(k)}$  in  $\mathcal{O}^{(k)}$  such that  $\mathcal{U}_a^{(k)} \subseteq \mathcal{O}_c^{(k)}$  and  $\mathcal{U}_b^{(k)} \subseteq \mathcal{O}_d^{(k)}$ . Since  $\{\mathcal{O}^{(1)}, \mathcal{O}^{(2)}, \dots, \mathcal{O}^{(K)}\}$  is a partition satisfying (8), condition (8) holds for any pair  $(x, y)$  where  $x \in \mathcal{U}_a^{(k)}$  ( $\mathcal{U}_a^{(k)} \subseteq \mathcal{O}_c^{(k)}$ ) and  $y \in \mathcal{U}_b^{(k)}$  ( $\mathcal{U}_b^{(k)} \subseteq \mathcal{O}_d^{(k)}$ ), which contradicts with the fact that there exist  $x' \in \mathcal{U}_a^{(k)}$  and  $y' \in \mathcal{U}_b^{(k)}$  such that condition (8) does not hold. That is, there exists one element  $\mathcal{O}_c^{(k)}$  in  $\mathcal{O}^{(k)}$  such that  $\mathcal{U}_a^{(k)} \subseteq \mathcal{O}_c^{(k)}$  and  $\mathcal{U}_b^{(k)} \subseteq \mathcal{O}_c^{(k)}$ . In this case, merging  $\mathcal{U}_a^{(k)}$  and  $\mathcal{U}_b^{(k)}$  would not violate (A22). This implies that if  $\{\mathcal{U}^{(1)}, \mathcal{U}^{(2)}, \dots, \mathcal{U}^{(K)}\}_i$  satisfies (A22), and then  $\{\mathcal{U}^{(1)}, \mathcal{U}^{(2)}, \dots, \mathcal{U}^{(K)}\}_{i+1}$  also satisfies (A22).

Our algorithm terminates when no groups can be merged. When our algorithm stops, it yields a partition  $\{\mathcal{U}^{(1)}, \mathcal{U}^{(2)}, \dots, \mathcal{U}^{(K)}\}$  finer than any  $\{\mathcal{O}^{(1)}, \mathcal{O}^{(2)}, \dots, \mathcal{O}^{(K)}\}$  satisfying condition (8). Therefore, the resultant  $\{\mathcal{U}^{(1)}, \mathcal{U}^{(2)}, \dots, \mathcal{U}^{(K)}\}$  is the finest partition satisfying condition (8), and by **Theorem 3**, it is the finest feasible partition satisfying condition (8).
